# Supplementary material for: Theory and Applications of Kernel Stein's Method on Riemannian Manifolds
Source: arXiv:2501.00695 source file (2025-06-10)
Supplement: Supplementary file 2 [file formulas_supp.tex]

\section{Formulas}

In practice we can compute $Q(X,Y)$ and $b(X,Y)$ elementwisely through a loop, or construct the  $N^2\times s$ matrix
$\mathcal{Z}(X):=(\vectz[\mathscr{A}(\nabla^\mathbb{R}_X\zeta_1 X^\top)],\dots,\vectz[\mathscr{A}(\nabla^\mathbb{R}_X\zeta_s X^\top)])  
$, then we have $
A(X,Y)=\kappa\cdot\mathcal{Z}(Y)^\top Z(X)$ and $ b(X,Y)=\kappa\cdot\mathcal{Z}(Y)^\top\vectz[\mathscr{A}(\nabla^\mathbb{R}_X\log(e^\eta\kappa)X^\top)]$. 

In practice we can compute $A(X,Y)$ and $b(X,Y)$ elementwisely through a loop, or construct the  $N^2\times s$ matrix
$\mathcal{Z}(X)=(\vectz[\mathscr{A}(\mathscr{S}(\nabla^\mathbb{R}_X\zeta_1) X)],\dots,\vectz[\mathscr{A}(\mathscr{S}(\nabla^\mathbb{R}_X\zeta_s) X)])  
$, then we have $
A(X,Y)=\kappa\cdot\mathcal{Z}(Y)^\top Z(X)$ and $ b(X,Y)=\kappa\cdot\mathcal{Z}(Y)^\top\vectz[\mathscr{A}(\mathscr{S}(\nabla^\mathbb{R}_X\log(e^\eta\kappa))X)]$. 

In practice we can compute $A(X,Y)$ and $b(X,Y)$ elementwisely through a loop, or construct the  $N^2\times s$ matrix
$\mathcal{Z}(X)=(\vectz[X\mathscr{S}(\nabla^\mathbb{R}_X\zeta_1)],\dots,\vectz[X\mathscr{S}(\nabla^\mathbb{R}_X\zeta_s) ])  
$, then we have $
A(X,Y)=\kappa\cdot\mathcal{Z}(Y)^\top Z(X)$ and $ b(X,Y)=\kappa\cdot\mathcal{Z}(Y)^\top\vectz[X\mathscr{S}(\nabla^\mathbb{R}_X\log(e^\eta\kappa))]$. We summarize into following theorem:

\subsection{Kp on Stiefel }
The $k_p$ function
\begin{itemize}
    \item ML-family with Gaussian kernel:
\begin{equation}\label{Stiefel-ML-kp}
\begin{aligned}
\kappa_F(X,Y)
&=\langle\mathscr{A}((F +\tau Y)X^\top), \mathscr{A}((F+\tau X)Y^\top) \rangle_{\F} \cdot \kappa(X,Y)\\
&+ \frac{\tau}{2}(N-1)\langle X, Y\rangle_{\F}\cdot \kappa(X,Y)
\end{aligned}
\end{equation}
\item MB-family with Gaussian kernel
\begin{equation}\label{Stiefel-MB-kp}
\begin{aligned}
\kappa'_A(X,Y) &=\langle\mathscr{A}((2 A X +\tau Y)X^\top)^\top \mathscr{A}((2 A Y+\tau X)Y^\top) \rangle_{\F} \cdot \kappa(X,Y)\\
&+ \frac{\tau}{2}(N-1)\langle X, Y\rangle_{\F} \kappa(X,Y)
\end{aligned}
\end{equation}
\item RG-family with Gaussian kernel
\begin{equation}\label{Stiefel-RG-kp}
\begin{aligned}
k_{\Bar{X},\varsigma}(X,Y)= &\tr[\mathscr{A}((\varsigma(I-\frac{1}{2}X X^\top)\Log_X(\Bar{X}) +\tau Y)X^\top)^\top\\
&\mathscr{A}((\varsigma(I-\frac{1}{2}Y Y^\top)\Log_Y(\Bar{X})+\tau X)Y^\top) ] \\
&\cdot e^{\tau \tr (X^\top Y)}+\frac{\tau}{2}(N-1)\tr(X^\top Y) e^{\tau \tr (X^\top Y)}.
\end{aligned}
\end{equation}
Here $\varsigma:=\sigma^{-2}$. 
\item ML-family with inverse quadratic kernel:
\begin{equation}
    \begin{aligned}
k_F(X,Y)
&=\tr[\mathscr{A}((F + \frac{2\gamma}{\beta+\Vert X-Y\Vert^2_{\tr}} Y)X^\top)^\top \mathscr{A}((F+ \frac{2\gamma}{\beta+\Vert X-Y\Vert^2_{\tr}} X)Y^\top)]\\
&\cdot (\beta+\Vert X-Y\Vert^2_{\tr})^{-\gamma} + \gamma(N-1)\tr(X^\top Y) \cdot (\beta+\Vert X-Y\Vert^2_{\tr})^{-\gamma-1}\\
&- 4\gamma\Vert\mathscr{A}(XY^\top)\Vert^2_{\tr}\cdot (\beta+\Vert X-Y\Vert^2_{\tr})^{-\gamma-2}
\end{aligned}
\end{equation}

\item MB-family with inverse quadratic kernel:
\begin{equation}
\begin{aligned}
k_A(X,Y)
&=\tr[\mathscr{A}((2AX + \frac{2\gamma}{\beta+\Vert X-Y\Vert^2_{\tr}} Y)X^\top)^\top \mathscr{A}((2AY+ \frac{2\gamma}{\beta+\Vert X-Y\Vert^2_{\tr}} X)Y^\top)]\\
&\cdot (\beta+\Vert X-Y\Vert^2_{\tr})^{-\gamma} + \gamma(N-1)\tr(X^\top Y) \cdot (\beta+\Vert X-Y\Vert^2_{\tr})^{-\gamma-1}\\
&- 4\gamma\Vert\mathscr{A}(XY^\top)\Vert^2_{\tr}\cdot (\beta+\Vert X-Y\Vert^2_{\tr})^{-\gamma-2}
\end{aligned}    
\end{equation}

\item RG-family with inverse quadratic kernel:
\begin{equation}
    \begin{aligned}
        k_{\Bar{X},\sigma}(X,Y)
&=\tr[\mathscr{A}((\varsigma(I-\frac{1}{2} X X^\top)\Log_X \Bar{X} + \frac{2\gamma}{\beta+\Vert X-Y\Vert^2_{\tr}} Y)X^\top)^\top\\
&\quad \mathscr{A}((\varsigma(I-\frac{1}{2} Y Y^\top)\Log_Y \Bar{X}+ \frac{2\gamma}{\beta+\Vert X-Y\Vert^2_{\tr}} X)Y^\top)]\cdot (\beta+\Vert X-Y\Vert^2_{\tr})^{-\gamma}\\
&+ \gamma(N-1)\tr(X^\top Y) \cdot (\beta+\Vert X-Y\Vert^2_{\tr})^{-\gamma-1}\\
&- 4\gamma\Vert\mathscr{A}(XY^\top)\Vert^2_{\tr}\cdot (\beta+\Vert X-Y\Vert^2_{\tr})^{-\gamma-2}
    \end{aligned}
\end{equation}
\end{itemize}

\subsection{MKSDE on Stiefel}
The MKSDEs are
\begin{itemize}
    \item ML-family with Gaussian kernel:
    \begin{equation}
    \begin{aligned}
    b(X,Y) &= \tau\vectz(\mathscr{A}( X Y^\top) X) \cdot e^{\tau\tr(X^\top Y)},
    \\  
    A(X,Y) &= \frac{1}{2 }  (I\otimes X Y^\top-S_{r,N}\cdot X\otimes Y^\top ) \cdot e^{\tau\tr(X^\top Y)},
\end{aligned}
    \end{equation}
    \item  MB-family with Gaussian kernel:
    \begin{equation}
        \begin{aligned}
    b(X,Y) &=  \tau\vectz(X Y^\top (X X^\top-I_N) ) e^{\tau\tr(X^\top Y)},
    \\
    A(X,Y) &= \frac{1}{2 } (S_{N,N}+I_{N^2}) (X X^\top Y Y^\top \otimes I_N -X X^\top \otimes Y Y^\top) (S_{N,N}+I_{N^2}) e^{\tau\tr(X^\top Y)},
        \end{aligned}
    \end{equation}
    \item ML-family with inverse quadratic kernel:
    \begin{equation}
    \begin{aligned}
    b(X,Y) &= 2\gamma (\beta+\Vert X-Y\Vert^2_{\tr})^{-\gamma-1} \vectz(\mathscr{A}(X Y^\top) X) \cdot k(X,Y),
    \\  
    A(X,Y) &= \frac{1}{2 } (\beta+\Vert X-Y\Vert^2_{\tr})^{-\gamma} (I\otimes X Y^\top-S_{r,N}\cdot X\otimes Y^\top ),
\end{aligned}
    \end{equation}
    \item MB-family with inverse quadratic kernel:
    \begin{equation}
    \begin{aligned}
    b(X,Y) &= 2\gamma (\beta+\Vert X-Y\Vert^2_{\tr})^{-\gamma-1}  \vectz(X Y^\top (X X^\top-I_N) ) k(X,Y),
    \\
    A(X,Y) &= \frac{1}{2 } (\beta+\Vert X-Y\Vert^2_{\tr})^{-\gamma}(S_{N,N}+I_{N^2}) (X X^\top Y Y^\top \otimes I_N -X X^\top \otimes Y Y^\top)\\ &\quad (S_{N,N}+I_{N^2}),
    \end{aligned}
    \end{equation}
\end{itemize}

\begin{corollary}[KSD] The $k_p$ functions for commonly-used families on $\mathcal{G}_r(N)$ are:
\begin{itemize}
    \item ML-family with Gaussian kernel:
    \begin{equation}\label{kp-Grassm-ML-Gauss}
    k_F(X,Y)
=4 \tr[\mathscr{A}((F +\tau Y)X)^\top \mathscr{A}((F+\tau X)Y) ] \cdot e^{\tau \tr (X Y)} + \tau(N\tr(XY)-r^2)e^{\tau\tr(XY)}.
\end{equation}
\item RG-family with Gaussian kernel:
\begin{equation}\label{kp-Grassm-RG-Gauss}
\begin{aligned}
k_{\Bar{X},\varsigma}(X,Y)= &\tr[\mathscr{A}((\varsigma\Log_X(\Bar{X}) + 2\tau Y)X)^\top \mathscr{A}((\varsigma\Log_Y(\Bar{X})+2\tau X\big)Y) ] \cdot e^{\tau \tr (X Y)}\\
&+ \tau(N\tr(XY)-r^2)e^{\tau\tr(XY)}.
\end{aligned}
\end{equation}
Here $\varsigma:=\sigma^{-2}$. 
\item ML-family with inverse quadratic kernel:
\begin{equation}\label{kp-Grassm-ML-inverse}
\begin{aligned}
k_F(X,Y)
&=4 \tr[\mathscr{A}((F +\tau Y)X)^\top \mathscr{A}((F+\tau X)Y) ] \cdot e^{\tau \tr (X Y)}\\
&+ 2\gamma(\beta+\Vert X-Y\Vert^2_{\tr})^{-\gamma-1}(N\tr(XY)-r^2)\\
&-4\gamma(\beta+\Vert X-Y\Vert^2_{\tr})^{-\gamma-2}]\Vert X-Y\Vert^2_{\tr}.
\end{aligned}
\end{equation}
\item RG-family with inverse quadratic kernel:
\begin{equation}\label{kp-Grassm-RG-inverse}
\begin{aligned}
k_{\Bar{X},\varsigma}(X,Y)= &\tr[\mathscr{A}((\varsigma\Log_X(\Bar{X}) + 2\tau Y)X)^\top \mathscr{A}((\varsigma\Log_Y(\Bar{X})+2\tau X\big)Y) ] \cdot e^{\tau \tr (X Y)}\\
&+ 2\gamma(\beta+\Vert X-Y\Vert^2_{\tr})^{-\gamma-1}(N\tr(XY)-r^2)\\
&-4\gamma(\beta+\Vert X-Y\Vert^2_{\tr})^{-\gamma-2}]\Vert X-Y\Vert^2_{\tr}.
\end{aligned}
\end{equation}
Here $\varsigma:=\sigma^{-2}$. 
\end{itemize}
\end{corollary}

\begin{corollary} The $k_p$ function for commonly-used families on $\mathcal{P}(N)$ are:
\begin{itemize}
    \item Wishart family: 
    \[
    \begin{aligned}
    k_{V,r}(X,Y)
&= \tr\big[(2\tau(Y-X) X+ (N-r+1)I- V^{-1}X )\\
&\quad  (2\tau Y(X-Y)+(N-r+1)I-YV^{-1})\big] \cdot e^{-\frac{\tau}{2}\Vert X-Y\Vert^2_{\tr}}\\
&+2\tau (N+1)\tr(X Y) e^{-\frac{\tau}{2}\Vert X-Y\Vert^2_{\tr}}.
    \end{aligned}
    \]
    \item Riemannian Gaussian family:
    \begin{equation}\label{SPD-RN-kp}
\begin{aligned}
k_{\Bar{X},\varsigma}(X,Y)
&= 4\tr\big[(\tau(Y-X) X-\Log(\Bar{X}^{-1} X) ) (\tau Y(X-Y)-\Log(\Bar{X}^{-1}Y) )\big] \\
&\quad \cdot e^{-\frac{\tau}{2}\Vert X-Y\Vert^2_{\tr}}+2\tau (N+1)\tr(X Y) e^{-\frac{\tau}{2}\Vert X-Y\Vert^2_{\tr}} 
\end{aligned}
\end{equation}
Here $\varsigma:=\sigma^{-2}$ and $\Log$ represents the matrix logarithm \cite[\S 2.1]{moakher2005differential}. 

\end{itemize}
\end{corollary}

\begin{proof} It suffices to calculate the Euclidean gradient $\nabla^\mathbb{R}_X\log p(X)$ for each family. For Wishart distribution, $\log p(X)=\frac{N-r+1}{2} \log |X|-\frac{1}{2}\tr[V^{-1} X]$. By the Jacobi's formula \cite[Thm. 8.1]{magnus2019matrix} $d|X|=|X|\tr(X^{-1} dX)$, we have $\nabla^\mathbb{R}_X \log p(X)= \frac{N-r+1}{2}  X^{-1}- \frac{1}{2} V^{-1} $. For the Riemannian Gaussian family, $\log p(X)=-\frac{\varsigma}{2} d^2(X,\Bar{X})$. As shown in \cite{moakher2005differential}, on $\mathcal{P}(N)$, $d^2(X,\Bar{X})=\tr(\Log^2(\Bar{X}^{-1}X))$. By proposition 2.1 in \cite{moakher2005differential}, we have 
\[
\frac{d}{d t} d^2(X(t),\Bar{X}) = \frac{d}{d t} \tr(\Log^2(\Bar{X}^{-1}X(t)))= 2\tr\left[\Log(\Bar{X}^{-1} X(t)) X^{-1}(t) \frac{d}{d t}X(t) \right].
\]
Therefore, $\nabla^\mathbb{R}_X \log p(X)= -X^{-1}\Log(\Bar{X}^{-1}X) $. 
\end{proof}

We will also encounter the gradient of a vector-valued function on $M$ in this section, as the function $\zeta:M\to \mathbb{R}^s$ in the exponential family $p_\theta\propto\exp(\theta^\top\zeta(X)+\eta(X))$ is vector-valued. Note that the gradient
$\nabla_X^\mathbb{R}\zeta$ will be a multidimensional (3D) array of dimension $s\times N\times r$, which can not be appropriately represented in matrix form. 
\[
(\vectz(\nabla_X \zeta_1 X^\top),\vectz(\nabla_X \zeta_1 X^\top),\cdots,\vectz(\nabla_X \zeta_s X^\top) )
\]

To tackle this issue, we vectorize the argument $X$, and define the function $\Vec{\zeta}:\mathbb{R}^{Nr}\to\mathbb{R}^s$ by letting $\Vec{\zeta}(\vectz(X))=\zeta(X)$ for $X\in\mathbb{R}^{N\times r}$, or equivalently, $\Vec{\zeta}(v)=\zeta(\vectz^{-1}(v))$ for $v\in\mathbb{R}^{N r}$. Then we let $\mathcal{Z}(X)=\nabla_v\Vec{\zeta}(v)|_{v=\vectz(X)}$. Note that
\[
\begin{aligned}
 \zeta(X+d X) 
 &=\Vec{\zeta}(\vectz(X+dX)) =\Vec{\zeta}(\vectz(X)+\vectz(d X))\\
 &=\Vec{\zeta}(\vectz(X))+\nabla_v\Vec{\zeta}(v)^\top|_{v=\vectz(X)} \cdot \vectz(d X)+o(d X)\\
 &= \zeta(X)+Z(X)^\top \cdot \vectz(d X)+o(d X).
\end{aligned}
\]
Furthermore, we have
\[
\begin{aligned}
\theta^\top Z(X)^\top \cdot \vectz(d X)+o(d X)
&=\theta^\top\zeta(X+d X)- \theta^\top\zeta(X)\\
(\text{definition of } \nabla^\mathbb{R}_X)\ 
&=\tr(\nabla^\mathbb{R}_X(\theta^\top \zeta(X))^\top\cdot d X)+ o(d X)\\
&=\vectz(\nabla^\mathbb{R}_X(\theta^\top \zeta(X))^\top \vectz(d X)+o(d X),
\end{aligned}
\]
which implies that $\vectz(\nabla^\mathbb{R}_X(\theta^\top\zeta(X)))=\mathcal{Z}(X)\theta$, or equivalently, $\nabla^\mathbb{R}_X(\theta^\top\zeta(X))=\vectz^{-1}(\mathcal{Z}(X)\theta)$. This equality will play an important role in the subsequent calculations.

\subsubsection{Kronecker Product, Vectorization and Shuffle matrix}
Let $A \otimes B$ represent the Kronecker product of two matrices $A\in\mathbb{R}^{N_1\times r_1}$ and $B\in\mathbb{R}^{N_2\times r_2}$.  The perfect shuffle matrix $S_{N,r}$ is a $Nr$ by $Nr$ matrix defined as
\begin{equation}
S_{N,r}=
\begin{bmatrix}
I_{Nr}(1:N:Nr,:)\\
I_{Nr}(2:N:Nr,:)\\
\vdots\\
I_{Nr}(N:N:Nr,:)
\end{bmatrix},    
\end{equation}
where $I_{Nr}$ is the $Nr\times Nr$ identity, and the Matlab colon notation is used here to indicate the submatrices. We refer the readers to \cite{van2000ubiquitous} for detailed definitions and properties of Kronecker product, vectorization and the shuffle matrix.
%\begin{proposition}   
We now list a few of the properties \cite{Graham,magnus1979commutation} that will be used subsequently in this work:
\begin{itemize}
    \item $A^\top\otimes B^\top = (A \otimes B)^\top$,
    \item $A\otimes(B\otimes C)=(A\otimes B)\otimes C$,
     \item $(A\otimes B)(C\times D)=(AC)\otimes (BD)$
    \item If $A,B$ are invertible, then $A\otimes B$ is invertible and $(A\otimes B)^{-1}=A^{-1}\otimes B^{-1}$.
    \item $ \vectz(BX A^\top)=(A\otimes B) \vectz(X) $.
    \item For $A\in\mathbb{R}^{N\times r}$, $\vectz(A^\top)=S_{N,r}\vectz(A)$.
    \item For $A\in\mathbb{R}^{N_1\times r_1}$ and $B\in\mathbb{R}^{N_2\times r_2}$, $S_{N_1,N_2}^\top (A\otimes B) S_{r_1,r_2}=(B\otimes A)$.
    \item $S_{N,r}^\top=S_{N,r}^{-1}=S_{r,N}$.
\end{itemize}
%\end{proposition}

\begin{theorem} If $h_\alpha(x,x)$ is $w$-integrable for all $\alpha$, then we have following inequalities almost surely:
\[
0\leq \varliminf_{n\to \infty} \inf_\alpha V^w_n(\alpha) \leq   \varlimsup_{n\to \infty} \inf_\alpha V^w_n(\alpha)\leq \inf_\alpha\ksd^2(p_\alpha,q),\quad \varlimsup_{n\to \infty} \inf_\alpha U^w_n(\alpha)\leq \inf_\alpha\ksd^2(p_\alpha,q).
\]
As a corollary, if $\inf_\alpha\ksd^2(p_\alpha,q)=0$, then $\inf_\alpha V^w_n(\alpha)\xrightarrow{a.s.}0$.
\end{theorem}

\begin{proof} First we prove the inequality for $V^w_n(\alpha)$. For the first "$\leq$", note that $(\kappa_{p_\alpha}(x_i,x_j))$ is a positive matrix, as $\kappa_{p_\alpha}(x,x')=\sum_{l=1}^m \langle (\mathcal{T}^l_{p_\alpha} \kappa)_x,(\mathcal{T}^l_{p_\alpha} \kappa)_{x'} \rangle_{\mathcal{H}_\kappa}$, which implies $V^w(\alpha) \geq 0$ for all $\alpha$.  The third "$\leq$" follows from the fact that $V^w_n(\alpha)\xrightarrow{a.s.} \ksd^2(p_\alpha,q)$, as we choose $\alpha_l$, $l>0$ such that $\ksd^2(p_{\alpha_l},q)\leq \inf_\alpha\ksd^2(p_\alpha,q)+ l^{-1}$ and then have
\[
\varlimsup_{n\to \infty} \inf_\alpha V^w_n(\alpha)\leq \varlimsup_{n\to \infty} V^w_n(\alpha_l) \leq \inf_\alpha\ksd^2(p_\alpha,q)+l^{-1}, \quad \text{for all } l>0,
\]
which concludes the result. The second inequality is directly from the fact that $U^w_n(\alpha)\leq V^w_n(\alpha)$.
\end{proof}
