# Supplementary material for: Theory and Applications of Kernel Stein's Method on Riemannian Manifolds
Source: arXiv:2501.00695 source file (2025-06-10)
Supplement: Supplementary file 3 [file mathbackground_supp.tex]

% \begin{center}
% {\huge \bf Supplement}
% \end{center}

% \begin{center}
% {\large Theory and Applications of Kernel Stein Discrepancy on Riemannian Manifolds 
% }
% \end{center}

% \begin{center}
% {\large Xiaoda Qu, Baba C. Vemuri}
% \end{center}
% \vspace{5mm}

% In this supplement we provide the necessary mathematical backgrounds that were omitted in the main text and the proofs to our theorems.

%\label{Riemannian-Geometry}
\section{Mathematical Background}\label{mathbackground_supp}
In this section, we set up the notations and standing assumptions, and then briefly introduce several mathematical definitions and concepts that will be used in the rest of the paper. For a more comprehensive study of the background material presented here, we refer the readers to some standard text books on  differential geometry \cite{lee2006riemannian,lee2013smooth,petersen2016riemannian}, reproducing kernel Hilbert spaces (RKHS) \cite{carmeli2010vector,steinwart2008support} and Bochner integral \cite[\S A.5.4]{steinwart2008support}.

\subsubsection*{Riemannian Geometry}

We begin by introducing smooth manifolds followed by tangent and cotangent tensors, then, Riemannian metric and distance. This is followed by the volume measure, the divergence theorem, Lie groups, Killing fields and finally Riemannian homogeneous spaces. 

\subsubsection*{Smooth Manifolds} A manifold $M$ is a second countable Hausdorff space that is locally homeomorphic to an open set in $\mathbb{R}^d$. The number $d$ is the \emph{dimension} of $M$. Such local homeomorphisms are called \emph{charts}. A smooth structure on $M$ is assigned via a collection of charts that covers the manifold such that the composition of every pair of charts of the collection is smooth on $\mathbb{R}^d$. A manifold with a smooth structure is called a \emph{smooth manifold}.

\subsubsection*{Tangent and Cotangent Vector} A \emph{local curve} at a point $x \in M$ is a smooth map $\mathfrak{c}:(-\epsilon,\epsilon)\to M $ with $\mathfrak{c}(0)=x$. A \emph{tangent vector} at $x$ is an equivalence class of local curves at $x$ with the same gradient $\frac{d}{d t}(\xi\circ \mathfrak{c})(0)$ for some chart $(U,\xi)$. The \emph{tangent space} $T_x M$ is the $n$-dimensional vector space of tangent vectors at $x \in M$. The \emph{cotangent space} $T_x^* M$ is then the dual space of $T_x M$. For a tangent vector $D_x\in T_x M$ and a smooth functions $f$, $D_x f$ represents the directional derivative of $f$ along $D_x$, defined via $D_x f=\frac{d }{d t} f\circ\mathfrak{c}(0)$ where $\mathfrak{c}$ is a local curve corresponding to $D_x$. A \emph{vector field} $D$ is a smooth assignment of vector fields to tangent spaces at each point, where $D_x$ represents the vector assigned to tangent space at $x$. For a map $f:M\to M'$ between two manifolds, the differential $df_x$ of $f$ at $x$ is defined as the map $df_x:T_x M\to T_{f(x)}M' $, $[\mathfrak{c}(t)]\to [f(\mathfrak{c}(t))] $, i.e, mapping the equivalence class of $\mathfrak{c}(t)$, which is a tangent vector in $T_xM$, to the equivalence class of $f(\mathfrak{c}(t))$, which is a tangent vector in $T_{f(x)}M'$.

\subsubsection*{Riemannian Metric and Distance}

A \emph{Riemannian metric} $g$ is a smooth assignment of inner product to tangent spaces at each point $x\in M$. A \emph{Riemannian manifold} $M$ is a smooth manifold endowed with a Riemannian metric $g$. For a connected Riemannian manifold $M$, any two points $x,y$ can be connected by a piecewise smooth curve $\gamma:[0,1]\to M$ with $\gamma(0)=x,\gamma(1)=y$. The length of the curve is then defined as $L(\gamma)=\int_0^1 |\gamma'(t)| d t $. The Riemannian distance $d$ is then given by 
$ d(x,y)=\inf \left\{L(\gamma):\text{for all } \gamma \text{ connecting } x,y\right\}$.
A Riemannian manifold \(M\) is called \emph{complete} if \((M,d)\) is a complete metric space. 

\subsubsection*{Volume Measure} The volume measure $\mu$ on $M$ can be defined as the $n$-dimensional Hausdorff measure or defined through integration of differential forms. These two definitions coincide.  For details we refer the readers to \cite{evans2018measure,lee2013smooth}. In this work, the readers are only required to know that the volume measure is the generalization of Euclidean Lebesgue measure to Riemannian manifolds, and commonly plays the role of a dominating measure of probability density functions on the manifolds.

\subsubsection*{Differential Operator} The Riemannian gradient operator $\nabla$ maps a smooth function $f$ to a smooth vector field $\nabla f$ such that $D(f)=g(D,\nabla f) $ for all smooth vector fields $D$. For the rather complicated definition of the divergence operator $\Div$, we refer the reader to \cite[\S 2.1.3]{petersen2016riemannian}. Very briefly, it maps a smooth vector field $D$ to a smooth function $\Div D$.  The divergence operator satisfies the property \cite[Exer. 2.5.5]{petersen2016riemannian} $\Div(fD)=Df+f\Div D$. 

% \begin{theorem}[Divergence theorem] \label{supp-DivThm} Let $M$ be a complete Riemannian manifold. For a locally Lipschitz continuous vector field $D$ on $M$ such that $|D|$ and $\Div D$ are both integrable w.r.t volume measure $\mu$, the following identity holds: \( \int_M \Div D d \mu= 0. \) 
% \end{theorem}
% \begin{proof} See \cite{gaffney1954special}.
% \end{proof}

\subsubsection*{Embedding}
A smooth map $\psi:M\to \mathbb{R}^{d'}$ for some $d'\geq d$ is said to be an \emph{smooth embedding} if $d\psi_x$ is injective for all $x\in M$ and $\psi$ is an homeomorphism between $M$ and $\psi(M)\subset\mathbb{R}^{d'}$ with subspace topology. Whitney embedding theorem \cite[Thm. 6.15]{lee2013smooth} shows that every smooth manifold admits a smooth embedding into higher dimensional Euclidean space.

\subsubsection*{Reproducing Kernel Hilbert Space}
In this section, we briefly introduce the reproducing kernel Hilbert space (RKHS) which will be needed later to define the kernel Stein discrepancy (KSD). For a detailed exposition on RKHS, we refer the readers to \cite{Manton} and \cite[\S 4]{steinwart2008support}.

A \emph{kernel function}, abbreviated as \emph{kernel} in this work, on a set $X$, is a bivariate function $\kappa:X\times X\to\mathbb{R}$ such that \begin{enumerate*}
    \item[(i)] symmetric, i.e., $\kappa(x,y)=\kappa(y,x)$ for all $x,y\in X$;
    \item[(ii)] positive definite, i.e., the matrix $(\kappa(x_i,x_j))_{i,j} \succeq 0$ for all $x_i\in X$, $1\leq i\leq n$.
\end{enumerate*}
It is widely known that (see e.g., \cite[Thm. 4.20 \& Thm. 4.21]{steinwart2008support}), for each kernel $\kappa$ on $X$, there exists an unique Hilbert space $\mathcal{H}_\kappa$, whose elements are real-valued functions on $X$, such that for each fixed $x_0\in X$, the uni-variate function $\kappa_{x_0}(\cdot):=\kappa(x_0,\cdot)$ belongs to $\mathcal{H}_\kappa$, and satisfies $f(x_0):=\langle f,\kappa_{x_0}\rangle_{\mathcal{H}_\kappa}$ for all $f\in \mathcal{H}_\kappa$. Specifically, note that $\kappa(x,y)=\langle \kappa_x,\kappa_y\rangle_{\mathcal{H}_\kappa}$. The function space $\mathcal{H}_\kappa$ is said to be the \emph{reproducing kernel Hilbert space (RKHS)} associated with kernel $\kappa$.

If $X$ is a locally compact topological space, we say a kernel $\kappa$ on $X$ is $C_0$ if $\mathcal{H}_\kappa\subset C_0(X)$, i.e., the space of continuous functions that vanish at infinity. Furthermore, a $C_0$ kernel $\kappa$ is said to be $C_0$-universal if $\mathcal{H}_\kappa$ is dense in $C_0(X)$ under the uniform norm. 
One type of the most widely-used $C_0$-universal kernels is the \emph{radial kernels}:

\subsubsection*{Bochner Integral} Given a probability space $(\Omega,\mathcal{F},P)$ and a separable Banach space $\mathcal{B}$, a $\mathcal{B}$-valued map $X:\Omega\to\mathcal{B}$ is said to be \emph{measurable} if $X^{-1}(B)$ is measurable for all Borel sets $B\subset\mathcal{B}$. A (measurable) step function is a map in the form of $X=\sum_{i=1}^m \textbf{1}_{A_i} x_i $ for some $x_1,\dots,x_n\in\mathcal{B}$ and $A_1,\dots,A_n\in\mathcal{F}$. For each measurable $\mathcal{B}$-valued map $X$, there exists a sequence of measurable step functions $X_n$ such that $\Vert X_n-X\Vert_{\mathcal{B}}\to 0 $ pointwisely. A measurable $\mathcal{B}$-valued map $X$ is \emph{Bochner $P$-integrable} if there exists a sequence of step functions $X_n=\sum_{i=1}^{m_n} \textbf{1}_{A_{i,n}}x_{i,n}$ such that $\lim_{n\to\infty} \mathbb{E}\Vert X_n-X\Vert=0$, then the expectation of $X$ is defined as $\mathbb{E} X=\lim_{n\to \infty} \sum_{i=1}^{m_n} P(A_{i,n}) x_{i,n} $. A measurable $\mathcal{B}$-valued map is $P$-integrable if and only if $\mathbb{E}\Vert X\Vert <+\infty$. For a detailed exposition on Bochner integral, we refer the readers to \cite[\S A.5.4]{steinwart2008support}. In addition, we have
\begin{theorem} Suppose $X$ is a $P$-integrable $\mathcal{B}$-valued map and $f$ is a continuous linear functional on $\mathcal{B}$, then $f(\mathbb{E}X)=\mathbb{E}f(X)$.
\end{theorem}
